# Supplementary material for: Extended black hole thermodynamics from extended Iyer-Wald formalism
Source: arXiv:2308.12630 ancillary file (2023-11-14)
Supplement: Supplementary file 1 [file attached_Notebook_PDF.pdf]

Note : The file uses the package "diffgeoM.m", which can be downloaded from : "<https://github.com/bryango/diffgeoM>".

## 1. The calculations for AdS -Schwarzschild black hole.

(0) The metric:

```
In[524]:= Quit[];
           退出内核

In[1]:= coord = {t, r,  $\theta$ ,  $\phi$ };
metricsign = -1;

metric = DiagonalMatrix[ $\left\{-1 + \frac{2M}{r} + \frac{r^2 \Lambda}{3}, \frac{1}{1 - \frac{2M}{r} - \frac{r^2 \Lambda}{3}}, r^2, r^2 \sin[\theta]^2\right\}$ ];
           对角矩阵

$Assumptions = And[M > 0, rh > 0, r > 0,  $\theta \geq 0$ ,  $\theta \leq \pi$ ,  $\phi \geq 0$ ,  $\phi < 2\pi$ ,  $\Lambda < 0$ ];
           默认假设           逻辑与

<< "D:\\diffgeoM.wl"
           偏导

tDelta[var_] := D[var, M] dM + D[var,  $\Lambda$ ] d $\Lambda$ ;
           偏导           偏导
```

(1) The computation of  $\int \tilde{\delta} Q$  on  $S_r$ :

```
In[7]:= xi = {1, 0, 0, 0};
xiD = lower[xi];
quvD = -1 / (16 Pi) * 2 * antisymmetrize[covariant[xiD]];
           圆周率

quv = raise[quvD, {1, 2}];
qXi = quv[[1, 2]] * 4 Pi r^2 // Expand;
           圆周率           展开

dQ = tDelta[qXi]
```

```
Out[12]=  $\frac{dM}{2} - \frac{d\Lambda r^3}{6}$ 
```

(2) The computation of  $-\int \xi \cdot \Theta$  on  $S_r$ : ( the minus sign is considered implicitly below)

```

In[13]:= ddMetric = covariant[tDelta[metric]];
1 / (16 Pi)
      [圆周率]
      (contract[ddMetric, {1, 3}] - contract[ddMetric, {2, 3}]) // Simplify;
      [化简]
xi ** raise[%, {1}];
xiTheta = %[[1, 2]] * 4 Pi r^2 // Expand
      [圆周率] [展开]

```

Out[16]=

$$\frac{dM}{2} + \frac{d\Lambda r^3}{3}$$

(3) Adding the results from (1) and (2), one gets  $\int \tilde{\delta} Q - \xi \cdot \Theta$  for the Killing vector  $\xi_t$  in the case of AdS-Schwarzschild black hole. Then regularize it by subtracting the pure AdS result. (Note that the substitution  $\{M \rightarrow 0, dM \rightarrow 0\}$  below gives the pure AdS result directly; alternatively, one can repeat the above calculation again directly starting from the metric of pure AdS.)

```

In[17]:= dQ + xiTheta;
% /. {M -> 0, dM -> 0};
%% - %

```

Out[19]=

$$dM$$

(4) **Verification of the extended first law** :  $dM = TdS + VdP$ . Below the expressions of  $M$ ,  $T$ ,  $S$ ,  $V$  are denoted by `mh`, `tem`, `entr` and `vol0`. When verifying the extended first law, we use the outer horizon radius  $r_h$  and the cosmological constant  $\Lambda$  as independent variables.

The expressions of the thermodynamic quantities are listed below: (As we emphasized in the paper, we do not need these expressions in deriving the extended 1st law, in sharp contrast to other approaches relying on the manipulations of thermodynamic relations. Whatever, one needs these expressions to do verification, in order to remove possible doubts.)

In[20]:=

```

mh =  $\frac{rh}{2} - \frac{rh^3 \Delta}{6}$ ; tem =  $\frac{1 - rh^2 \Delta}{4 \pi rh}$ ;

entr = Pi rh^2;
      [圆周率]

-2 Pi Integrate[rg, {θ, 0, Pi}, {r, rh, ifty}];
      [积分] [圆周率]

% /. {m → 0, rh → 0};
vol0 = %% - % // Simplify
      [化简]

```

Out[24]=

$$\frac{4 \pi rh^3}{3}$$

The verification:

In[25]:=

```

va = {rh, Δ};
For[i = 1, i ≤ 2, i++, Print[Simplify[
      [For循环] [打印] [化简]

      D[mh, va[[i]]] - tem * D[entr, va[[i]]] - (vol0) * D[ $-\frac{\Delta}{8 \pi}$ , va[[i]]] == 0]
      [偏导] [偏导]

]]

```

True

True

## 2. The calculations for AdS-Kerr black hole.

(0) The metric:

(The scale  $l$  is the AdS radius, with  $\ell^2 = -\frac{3}{\Lambda}$  and  $dl = \frac{3}{2l\Lambda^2} d\Lambda$  in D=4 dimensions.)

In[27]:=

```

Quit[];
[退出内核]

```

In[1]:=

```
metricKerr = { { (-a^2 (1^2 + r^2) - r (r^3 + 1^2 (-2 m + r)) + (a^2 1^2 - a^4 Cos[θ]^2) Sin[θ]^2) /
  (1^2 (r^2 + a^2 Cos[θ]^2)), 0, 0,
  - ( (a (r (-2 1^2 m + a^2 r + r^3) + a^2 (a^2 + r^2) Cos[θ]^2) Sin[θ]^2) /
    ((a^2 - 1^2) (r^2 + a^2 Cos[θ]^2))) },
  { 0, 0,  $\frac{r^2 + a^2 \cos[\theta]^2}{-2 m r + (a^2 + r^2) \left(1 + \frac{r^2}{1^2}\right)}$ , 0 }, { 0, 0,  $\frac{r^2 + a^2 \cos[\theta]^2}{1 - \frac{a^2 \cos[\theta]^2}{1^2}}$ , 0 },
  { - ( (a (r (-2 1^2 m + a^2 r + r^3) + a^2 (a^2 + r^2) Cos[θ]^2) Sin[θ]^2) /
    ((a^2 - 1^2) (r^2 + a^2 Cos[θ]^2))) , 0, 0,
    ( Sin[θ]^2 ( (a^2 + r^2)^2 (1 -  $\frac{a^2 \cos[\theta]^2}{1^2}$ ) - a^2 (-2 m r + (a^2 + r^2) (1 +  $\frac{r^2}{1^2}$ )) Sin[θ]^2) ) /
    ( (-1 +  $\frac{a^2}{1^2}$ )^2 (r^2 + a^2 Cos[θ]^2) ) ) } }
```

In[2]:=

```
coord = {t, r, θ, ϕ};
metricsign = -1;
metric = metricKerr;
$Assumptions =
默认假设
And[m > 0, rh > 0, r > 0, θ ≥ 0, θ ≤ π, ϕ ≥ 0, ϕ < 2 π, Δ < 0, 1 > a, a > 0];
逻辑与
<< "D:\\diffgeom.wl"
偏导
```

In[7]:=

```
tDelta[var_] := D[var, m]  $\frac{\partial}{\partial m}$  + D[var, a]  $\frac{\partial}{\partial a}$  + D[var, l]  $\frac{\partial}{\partial l}$ ;
tDelta1[var_] := D[var, m]  $\frac{\partial}{\partial m}$ ; tDelta2[var_] := D[var, a]  $\frac{\partial}{\partial a}$ ;
tDelta3[var_] := D[var, l]  $\frac{\partial}{\partial l}$ ;
```

(1) The computation of  $\int \tilde{\delta} \mathbf{Q}$  on  $S_r$  for the Killing vector  $\xi_t = d/dt - \frac{a}{1^2} d/d\phi$  conjugate to the energy. Below the contributions from the vector  $d/dt$  and the vector  $d/d\phi$  are calculated separately and are added together eventually.

```
In[10]:= xi1 = {1, 0, 0, 0};
xiD = lower[%];
quvD = -1 / (16 Pi) × 2 * antisymmetrize[covariant[%]];
quv = raise[%, {1, 2}];
qXi1 = 2 Pi Integrate[%[[1, 2]] * rg, {0, 0, Pi}];
dQ1 = tDelta[%] // Simplify;
```

```
In[16]:= xi2 = {0, 0, 0, 1};
xiD = lower[%];
quvD = -1 / (16 Pi) × 2 * antisymmetrize[covariant[%]];
quv = raise[%, {1, 2}];
qXi2 = 2 Pi Integrate[%[[1, 2]] * rg, {0, 0, Pi}];
dQ2 = tDelta[%];
dQ = dQ1 -  $\frac{a}{1^2}$  dQ2 // Simplify;
```

Out[22]=

$$\frac{1}{2 (a-1)^3 (a+1)^3} \left( -dm l^6 + 2 dl l^3 r^3 + a^4 l (dm l + 6 dl m - 2 dl r) + 2 a^3 da (r^3 + l^2 (-2m + r)) + 2 a^2 dl l (-r^3 + l^2 (m + r)) - 2 a da l^2 (r^3 + l^2 (2m + r)) \right)$$

(2) The computation of  $-\int \xi \cdot \Theta$ : the minus sign is considered implicitly below. The three parts proportional to  $\tilde{\delta}m$ ,  $\tilde{\delta}a$  and  $\tilde{\delta}l$  are calculated separately, and afterwards we add them together.

```
In[23]:= ddMetric = covariant[tDelta1[metric]];
1 / (16 Pi) (contract[ddMetric, {1, 3}] - contract[ddMetric, {2, 3}]);
(xi1 -  $\frac{a}{1^2}$  xi2) ** raise[%, {1}];
xiTheta1 = 2 Pi Integrate[Simplify[%[[1, 2]] * rg], {0, 0, Pi}];
```

```
In[27]:= ddMetric = covariant[tDelta2[metric]];
1 / (16 Pi) (contract[ddMetric, {1, 3}] - contract[ddMetric, {2, 3}]);
(xi1 -  $\frac{a}{1^2}$  xi2) ** raise[%, {1}];
xiTheta2 = 2 Pi Integrate[Simplify[%[[1, 2]] * rg], {0, 0, Pi}];
```

```

In[31]:= ddMetric = covariant[tDelta3[metric]];
1 / (16 Pi) (contract[ddMetric, {1, 3}] - contract[ddMetric, {2, 3}]);
      [圆周率]

(x11 -  $\frac{a}{1^2}$  x12) ** raise[%, {1}];
xiTheta3 = 2 Pi Integrate[Simplify[% [1, 2]] * rg], {0, 0, Pi}];
      [...] [积分] [化简] [圆周率]
xiTheta = xiTheta1 + xiTheta2 + xiTheta3 // Simplify;
      [化简]

```

(3) Adding the results from (1) and (2), one gets  $\int \delta Q - \xi \cdot \Theta$  for the Killing vector  $\xi_t$  in the case of AdS-Kerr black hole. Then regularize it by subtracting the pure AdS result.

```

In[36]:= dQ + xiTheta;
% /. {m -> 0, dm -> 0};
%% - % // Simplify;
      [化简]
dqXi = Limit[%, r -> Infinity];
      [极限] [无穷大]
Coefficient[%, dm] dm + Coefficient[%, da] da + Coefficient[%, dl] dl
      [系数] [系数]

```

Out[40]=

$$\frac{dm (a^2 l^4 - l^6)}{(a-1)^3 (a+1)^3} - \frac{4 a da l^4 m}{(a-1)^3 (a+1)^3} + \frac{dl (a^4 l m + 3 a^2 l^3 m)}{(a-1)^3 (a+1)^3}$$

When studying **conventional** thermodynamics where  $\delta l=0$ , the above expression is integrable. It gives  $\delta M = \delta \left( \frac{m}{\left(1 - \frac{a^2}{l^2}\right)^2} \right)$ . So we identify the conventional

1st law:  $\delta M - \Omega \delta J - T \delta S = 0$ .

But when studying the **extended** thermodynamics where  $\delta l$  does not vanish, the above expression is **not integrable** any more. It gives  $\tilde{\delta M} - \frac{4\pi}{3} M a^2 \tilde{\delta P}$ .

So we identify the extended 1st law:  $\delta M - \Omega \delta J - T \delta S = (V + \frac{4\pi}{3} M a^2) \tilde{\delta P}$ .

Below is the verification of that  $\int \delta Q - \xi \cdot \Theta$  produces  $\tilde{\delta M} - \frac{4\pi}{3} M a^2 \tilde{\delta P}$ :

```

In[41]:= dqXi ==
      tDelta[ $\frac{m}{(1 - a^2 / l^2)^2}$ ] -  $\frac{4 \pi}{3} \frac{m}{(1 - a^2 / l^2)^2} a^2$  tDelta[ $\left(-\frac{\Lambda}{8 \pi} / . \Lambda \rightarrow -\frac{3}{l^2}\right)$ ];
% // Simplify
      [化简]

```

Out[42]=

True

(4) **Verification of the extended first law.** Below the expressions of M, T, S, J,  $\Omega$ , V are denoted by mh, tem, entr, jh, omeg and vol0 . When verifying the extended first law, we use the outer horizon radius  $r_h$ , the rotating parameter a and the AdS radius l as independent variables.

The expressions of the thermodynamic quantities are listed below : (As we emphasized, we do not need these expressions in deriving the thermodynamic volume  $V^{\text{th}}=V+\Delta V$  and the extended 1st law. But in case that one is doubtful with our results, these expressions are needed to do verification.)

```
In[43]:=
m0 = 
$$\frac{(a^2 + r h^2) (l^2 + r h^2)}{2 l^2 r h}$$
; mh = m0 /  $(1 - a^2 / l^2)^2$ ;
jh = mh a; entr =  $\text{Pi} \frac{l^2 (a^2 + r h^2)}{a^2 + l^2}$ ;
tem = 
$$\frac{a^2 (-l^2 + r h^2) + r h^2 (l^2 + 3 r h^2)}{4 l^2 \pi r h (a^2 + r h^2)}$$
;
omeg = a (1 + r h^2 / l^2) / (r h^2 + a^2);

-2 Pi Integrate[rg, {0, 0, Pi}, {r, rh, ifty}];
% /. {m -> 0, rh -> 0};
vol0 = %% - % // Simplify
```

```
Out[49]=

$$\frac{4 l^2 \pi r h (a^2 + r h^2)}{3 (-a^2 + l^2)}$$

```

The verification:

```
In[50]:=
va = {rh, a, l};
For[i = 1, i <= 3, i++,
Print[Simplify[D[mh, va[[i]]] - omeg D[jh, va[[i]]] - tem * D[entr, va[[i]]] -
(vol0 +  $\frac{4 \text{Pi}}{3} mh * a^2$ ) * D[ $-\frac{\Lambda}{8 \text{Pi}}$  /.  $\Lambda \rightarrow -\frac{3}{l^2}$ ], va[[i]]] == 0]
]]
```

True

True

True

### 3. The calculations for the static and spherical black hole in higher curvature gravity that contains $O(R^2)$ and $O(R^3)$ terms in the action.

(0) The metric:

Below we use  $\gamma a_2$  and  $\gamma a_3$  to replace  $a_2$  and  $a_3$ , where  $\gamma$  is assumed to be a small quantity. So we can expand the computed results up to  $\gamma^2$ , which gives the 2nd order results.

(We have solved the black hole solution perturbatively around the AdS-Schwarzschild metric in the given higher curvature theory. The integration constants have been chosen to fix M as the canonical energy of the system. This choice simplifies the subsequent analysis. Otherwise, M should be regarded as an ordinary mass parameter, and it requires some special attention to be paid to the integrability condition when studying the extended black hole thermodynamics.)

In[52]:=

Quit[];  
退出内核

In[1]:=

```
metric = {{-a[r], 0, 0, 0}, {0, 1/b[r], 0, 0}, {0, 0, r^2, 0}, {0, 0, 0, r^2 Sin[θ]^2}};

af[r_] := 1 - 2 M/r - r^2 Λ/3 + γ (640 a3 M^3 π / r^7 - 256 a3 M^2 π Λ / r^4 - 128 a3 M π Λ^2 / (3 r) - 64 a3 π r^2 Λ^3 / 27) +
1 / (891 r^13) 4096 γ^2 (7 107 507 a3^2 M^5 π^2 - 6 980 904 a3^2 M^4 π^2 r + 1 679 616 a3^2 M^3 π^2 r^2 -
1 058 508 a2 a3 M^4 π^2 r^3 + 1 010 394 a2 a3 M^3 π^2 r^4 - 240 570 a2 a3 M^2 π^2 r^5 + 57 024 a3^2 M^4
π^2 r^3 Λ + 1 011 852 a3^2 M^3 π^2 r^4 Λ - 481 140 a3^2 M^2 π^2 r^5 Λ - 304 722 a2 a3 M^3 π^2 r^6 Λ +
144 342 a2 a3 M^2 π^2 r^7 Λ - 462 132 a3^2 M^3 π^2 r^6 Λ^2 + 288 684 a3^2 M^2 π^2 r^7 Λ^2 - 21 384
a2 a3 M^2 π^2 r^9 Λ^2 - 46 728 a3^2 M^2 π^2 r^9 Λ^3 - 330 a3^2 M π^2 r^12 Λ^4 - 11 a3^2 π^2 r^15 Λ^5);

bf[r_] := 1 - 2 M/r - r^2 Λ/3 - 1 / (27 r^7) 64 γ (2646 a3 M^3 π - 1458 a3 M^2 π r +
594 a3 M^2 π r^3 Λ + 18 a3 M π r^6 Λ^2 + a3 π r^9 Λ^3) - 1 / (891 r^13) 4096 γ^2
(1 649 241 a3^2 M^5 π^2 - 997 272 a3^2 M^4 π^2 r - 96 228 a2 a3 M^4 π^2 r^3 + 48 114 a2 a3 M^3 π^2 r^4 +
648 648 a3^2 M^4 π^2 r^3 Λ - 96 228 a3^2 M^3 π^2 r^4 Λ + 16 038 a2 a3 M^3 π^2 r^6 Λ -
16 038 a2 a3 M^2 π^2 r^7 Λ + 226 908 a3^2 M^3 π^2 r^6 Λ^2 - 80 190 a3^2 M^2 π^2 r^7 Λ^2 +
5346 a2 a3 M^2 π^2 r^9 Λ^2 + 32 472 a3^2 M^2 π^2 r^9 Λ^3 + 330 a3^2 M π^2 r^12 Λ^4 + 11 a3^2 π^2 r^15 Λ^5)

sr[va_] := Normal[Series[va, {γ, 0, 2}]];
```

转换... 级数

Above, af[r] and bf[r] are the concrete expressions of a[r] and b[r]. We do



the substitution  $a \rightarrow af$ ,  $b \rightarrow bf$  when it is needed.

In[4]:=

```
coord = {t, r,  $\theta$ ,  $\phi$ };
metricsign = -1;
metric;
$Assumptions = And[M > 0, rh > 0, r > 0,  $\theta \geq 0$ ,  $\theta \leq \pi$ ,  $\phi \geq 0$ ,  $\phi < 2\pi$ ,  $\Lambda < 0$ ];
默认假设 逻辑与
<< "D:\\diffgeoM.wl"
偏导
rie0 = lower[Riemann, {4}];
```

In[10]:=

```
tDelta[var_] := D[var, M] dM + D[var,  $\Lambda$ ] d $\Lambda$  + D[var, a2] da2 + D[var, a3] da3;
偏导 偏导 偏导 偏导
```

(1) We calculate  $\tilde{\delta}q$  on  $S_r$  for the Killing vector  $\xi_t = d/dt$  conjugate to the energy.

In higher curvature gravity, the expressions for  $Q$  and  $\Theta$  depend on the derivative of the Lagrangian with respect to Riemann curvature, which we shall denote as  $eof$ . We calculate its concrete expression for the present model as below.

In[11]:=

```
1 / (16 Pi) Transpose[inverse ** inverse, {1, 3, 2, 4}];
... 转置
eof1 = 1 / 2 (% - Transpose[%, {2, 1, 3, 4}]) // Simplify;
转置 化简
2 a2  $\gamma$  rie0;
3 a3  $\gamma$  contract[rie0 ** rie0, {1, 7}, {2, 8}];
eof2 = raise[%% + %, {1, 2, 3, 4}];
eof = eof1 + eof2;
```

In higher curvature theory,  $q$  includes two parts:  $Q^{ab} = -2 eof^{abcd} n_{ab} + 4 \xi_d \nabla_c eof^{abcd}$ , which we calculate separately and add together below.

In[24]:=

```
xi1 = {1, 0, 0, 0};
xiD = lower[%];
dxi = covariant[%];
tr[-2 eof ** dxi, {3, 5}, {4, 6}] // Simplify;
化简
% /. {a  $\rightarrow$  af, b  $\rightarrow$  bf} // sr;
%[[1, 2]] * 4 Pi r^2 *  $\sqrt{af[r] / bf[r]}$  // sr;
圆周率
qXiPart1 = % // Simplify // Expand;
化简 展开
```

```

In[31]:= lower[eof, {1, 2, 3, 4}];
covariant[%];
contract[%, {1, 5}];
raise[%, {1, 2, 3}];
-4 %.xiD;
% /. {a → af, b → bf} // sr;
%[[1, 2]] * 4 Pi r^2 *  $\sqrt{af[r] / bf[r]}$  // sr;
⌈圆周率
qXiPart2 = % // Simplify // Expand;
⌈化简 ⌈展开

```

```

In[39]:= qXi = qXiPart1 + qXiPart2 // Simplify;
⌈化简
dQ = tDelta[qXi] // sr;

```

(2) We calculate  $-\int \xi \cdot \Theta$  below: the minus sign is considered implicitly. In higher curvature gravity,  $\Theta = 2 \text{ eof}^{abcd} \nabla_d \delta g_{bc} - 2 \nabla_d \text{ eof}^{abcd} \delta g_{cd}$ . We calculate the two parts separately and add them together.

```

In[41]:= dMetric[r_] = {{ad[r], 0, 0, 0}, {0, bd[r], 0, 0}, {0, 0, 0, 0}, {0, 0, 0, 0}};
ddMetric = covariant[dMetric[r]];
adf[r_] = tDelta[-af[r]];
bdf[r_] = tDelta[1 / bf[r]];

```

```

In[45]:= 2 tr[efof.ddMetric, {2, 4}, {3, 5}] // Simplify;
⌈化简
xiThetaPart1 = %[[2]] /. {a → af, b → bf, ad → adf, bd → bdf} // sr;
xiTheta1 = % * 4 Pi r^2 *  $\sqrt{af[r] / bf[r]}$  // sr;
⌈圆周率

```

```

In[48]:= lower[efof, {1, 2, 3, 4}];
covariant[%];
contract[%, {1, 5}];
raise[%, {1, 2, 3}];
-2 % ** dMetric[r];
tr[%, {2, 4}, {3, 5}];
xiThetaPart2 = %[[2]] /. {a → af, b → bf, ad → adf, bd → bdf} // sr;
xiTheta2 = % * 4 Pi r^2 *  $\sqrt{af[r] / bf[r]}$  // sr;
⌈圆周率

```

```

In[56]:= xiTheta = xiTheta1 + xiTheta2 // Simplify // sr;
⌈化简

```

(3) Adding the results from (1) and (2), we get  $\int \delta Q - \xi \cdot \Theta$  for the Killing vec-

tor  $\xi_t$  in the present case. Then regularize it by subtracting the results for the pure AdS.

In[57]:=

```
dQ + xiTheta;
dqXi = Coefficient[%, dM] dM + Coefficient[%, dΛ] dΛ +
      Coefficient[%, da2] da2 + Coefficient[%, da3] da3;
```

In[59]:=

```
dqXi;
% /. {M → 0, dM → 0};
Limit[Simplify[% - %], r → Infinity];
dqXiReg = Coefficient[%, dM] dM + Coefficient[%, dΛ] dΛ +
          Coefficient[%, da2] da2 + Coefficient[%, da3] da3;
```

Out[62]:=

$$dM + da2 \left( -\frac{32}{3} M \pi \gamma \Lambda - \frac{8192}{27} a3 M \pi^2 \gamma^2 \Lambda^3 \right) + da3 \left( -\frac{32}{3} M \pi \gamma \Lambda^2 - \frac{10240}{27} a3 M \pi^2 \gamma^2 \Lambda^4 \right)$$

(4) **Verification of the extended first law.** Below the expressions of  $M$ ,  $T$ ,  $S$ ,  $V$ ,  $V_2$ ,  $V_3$  are denoted by  $mh$ ,  $tem$ ,  $entr$ ,  $vol0$ ,  $vol2$ ,  $vol3$ . When verifying the extended 1st law, we use the outer horizon radius  $r_h$ , the cosmological constant  $\Lambda$ , the couplings  $a_2$  and  $a_3$  as independent variables.

The expressions of the thermodynamic quantities are listed below: (For the convenience of the readers, starting from the metric, we have derived the expressions of the mass, temperature and entropy from standard techniques. The entropy is computed from Wald entropy formula.)

In[63]:=

$$\begin{aligned}
mh &= \frac{rh}{2} - \frac{rh^3 \Lambda}{6} + a3 \gamma \left( \frac{40 \pi}{rh^3} - \frac{72 \pi \Lambda}{rh} + 24 \pi rh \Lambda^2 - \frac{8}{3} \pi rh^3 \Lambda^3 \right) + \\
&\quad \gamma^2 \left( -\frac{1728 a3^2 \pi^2}{11 rh^7} - \frac{29376 a3^2 \pi^2 \Lambda}{11 rh^5} + \frac{41088 a3^2 \pi^2 \Lambda^2}{11 rh^3} - \right. \\
&\quad \left. \frac{26496 a3^2 \pi^2 \Lambda^3}{11 rh} + \frac{25280}{33} a3^2 \pi^2 rh \Lambda^4 - \frac{832}{9} a3^2 \pi^2 rh^3 \Lambda^5 \right); \\
tem &= \frac{1 - rh^2 \Lambda}{4 \pi rh} + \gamma \left( -\frac{12 a3}{rh^5} - \frac{12 a3 \Lambda}{rh^3} + \frac{12 a3 \Lambda^2}{rh} - 4 a3 rh \Lambda^3 \right) - \\
&\quad \frac{1}{33 rh^9} 32 \gamma^2 \left( 1809 a3^2 \pi - 4509 a3^2 \pi rh^2 \Lambda + 3402 a3^2 \pi rh^4 \Lambda^2 - \right. \\
&\quad \left. 450 a3^2 \pi rh^6 \Lambda^3 - 395 a3^2 \pi rh^8 \Lambda^4 + 143 a3^2 \pi rh^{10} \Lambda^5 \right); \\
entr &= \pi rh^2 + \gamma 64 a2 \pi^2 + \gamma \frac{192 a3 \pi^2}{rh^2};
\end{aligned}$$

In[66]:=

```

4 Pi r^2 Sqrt[af[r] / bf[r]] // sr;
(* 圆周率 *)
int[r_] = Integrate[%, r];
(* 积分 *)
- (int[r] - int[rh]) + (int[r] /. M -> 0) // sr;
Limit[%, r -> Infinity] // sr;
(* 无穷大 *)
vol0 = % // sr;

```

In[71]:=

```

gamma rie0 ** rie0;
contract[%, {3, 5}, {4, 6}];
contract[%, {1, 3}, {2, 4}];
4 Pi r^2 Sqrt[af[r] / bf[r]] * % /. {a -> af, b -> bf} // sr;
(* 圆周率 *)
int[r_] = Integrate[%, r];
(* 积分 *)
- (int[r] - int[rh]) + (int[r] /. M -> 0) // sr;
Limit[%, r -> Infinity] // sr;
(* 无穷大 *)
vol2 = % // sr;

```

```

In[79]:= γ rie0 ** rie0;
contract[%, {3, 5}, {4, 6}];
contract[%** rie0, {3, 5}, {4, 6}];
contract[%, {1, 3}, {2, 4}];
4 Pi r^2 √af[r] / bf[r] * % /. {a → af, b → bf} // sr;
⌈圆周率
int[r_] = Integrate[%, r];
⌈积分
- (int[r] - int[rh]) + (int[r] /. M → 0) // sr;
Limit[%, r → Infinity] // sr;
⌈极限 ⌈无穷大
vol3 = % // sr;

```

Verification of the extended first law :

```

In[88]:= va = {rh, Λ, a2, a3};
For[i = 1, i ≤ 4, i++,
⌈For循环
Print[sr[D[mh, va[[i]]] - (tem * D[entr, va[[i]]] + vol0 * D[-Λ/(8 Pi), va[[i]]] +
⌈打印 ⌈偏导 ⌈偏导 ⌈偏导
( vol12 + (32/3 M π γ Λ + 8192/27 a3 M π² γ² Λ³) ) D[a2, va[[i]]] +
( (vol13 + (32/3 M π γ Λ² + 10240/27 a3 M π² γ² Λ⁴) ) D[a3, va[[i]]] ) /. M →
⌈偏导
mh) == 0]]]

```

True

True

True

True

(5) **Verification of the correlation between  $\Delta M$  and  $\Delta V_n$** . Below we verify the correlation between the additional terms  $\Delta M = M - M_K$  and  $\Delta V_n$ , as suggested in the paper:

```

In[90]:= 2 qXi;
% /. M → 0;
%% - % // sr;
MK = Limit[%, r → Infinity] // sr;
⌈极限 ⌈无穷大

```

In[94]:= 
$$2 a2 \left( \frac{32}{3} M \pi \gamma \Lambda + \frac{8192}{27} a3 M \pi^2 \gamma^2 \Lambda^3 \right) + 4 a3 \left( \frac{32}{3} M \pi \gamma \Lambda^2 + \frac{10240}{27} a3 M \pi^2 \gamma^2 \Lambda^4 \right);$$
  
`Simplify[M - MK == %]`  
 化简

Out[95]= True

(6) One can use the **effective cosmological constant**  $\Lambda_e$  to rewrite the first law.

In[96]:= `af[r] /. M -> 0`  
`bf[r] /. M -> 0;`

Out[96]= 
$$1 - \frac{r^2 \Lambda}{3} - \frac{64}{27} a3 \pi r^2 \gamma \Lambda^3 - \frac{4096}{81} a3^2 \pi^2 r^2 \gamma^2 \Lambda^5$$

From it, you can read off the expression of  $\Lambda_e$  as a function of  $\Lambda$ ,  $a2$ ,  $a3$ , up to 2nd order, which is given by

In[98]:= 
$$\Lambda_{ef} = \Lambda \left( 1 + \frac{64}{9} a3 \pi \gamma \Lambda^2 + \frac{4096}{27} a3^2 \pi^2 \gamma^2 \Lambda^4 \right);$$

Conversely, you can also solve the expression of  $\Lambda$  as a function of  $\Lambda_e$ ,  $a2$ ,  $a3$ , up to 2nd order, which is given by

In[99]:= 
$$\Delta f = \Delta e + \gamma a3 \left( -\frac{64 \pi \Lambda e^3}{9} \right);$$

(This expression is exact up to 2nd order. The coefficient of  $\gamma^2$  happens to be 0.)

Thus, the term  $d\Lambda$  in the extended the first law can be replaced by the terms proportional to  $d\Lambda_e$ ,  $da2$ , and  $da3$ :

In[100]:= `D[Δf, Δe] dΔe + D[Δf, a2] da2 + D[Δf, a3] da3;`  
 偏导 偏导 偏导

4. The calculations for the spherically symmetric black hole in Lovelock gravity in D=5 dimensions (where only the Gauss-Bonnet term are involved):

(0) The metric:

In[10]:= **Quit[];**  
退出内核

In[1]:= **metric = DiagonalMatrix[**  
对角矩阵  
**{-(f[r]), 1/(f[r]), r^2, r^2\*(Sin[ψ])^2, r^2\*(Sin[ψ]\*Sin[θ])^2}];**  
正弦 正弦 正弦  
$$\text{fff}[r_] = 1 + \frac{r^2 \left( 1 - \sqrt{1 - \frac{8\alpha}{l^2} + \frac{64 M \alpha}{3 \pi r^4}} \right)}{4 \alpha};$$

Above, fff[r] is the concrete expression of f[r]. We do the substitution  $f \rightarrow \text{fff}$  when it is needed. The cosmological constant  $\Lambda$  and the AdS radius  $l$  are related by:  $\Lambda = -\frac{6}{l^2}$  in  $D = 5$  dimensions.

In[3]:= **coord = {t, r, ψ, θ, φ};**  
**metricsign = -1;**  
  
**\$Assumptions = And[t ∈ Reals, M ∈ Reals, r ∈ Reals, r > 0,**  
默认假设 逻辑与 实数域 实数域 实数域  
**0 < φ < 2 π, 0 < ψ < π, 0 < θ < π, M > 0, α > 0, rh > 0, l > 0];**  
**<< "D:\\diffgeoM.wl"**  
偏导  
**rie0 = lower[Riemann, {4}];**

In[8]:= **tDelta[var\_] := D[var, M] dM + D[var, l] dl + D[var, α] dα;**  
偏导 偏导 偏导

(1) We calculate  $\tilde{\delta} Q$  on  $S_r$  for the Killing vector  $\xi_t = d/dt$  conjugate to the energy.

In higher curvature gravity, the expressions for  $Q$  and  $\Theta$  depend on the derivative of the Lagrangian with respect to Riemann curvature, which we shall denote as **eof**. Below we calculate its concrete expression for the present model.

In[9]:= **metric \*\* metric + α (-4 \* 2 metric \*\* RicciTensor + 2 metric \*\* metric RicciScalar);**  
**Transpose[%, {1, 3, 2, 4}] + α 2 rie0;**  
转置  
**antisymmetrize[antisymmetrize[%, {1, 2}], {3, 4}];**  
**eof = raise[ $\frac{1}{16 \pi}$  \* %, {1, 2, 3, 4}] // Simplify;**  
化简

In higher curvature theory,  $q$  includes two parts:  $Q^{ab} = -2 \text{eof}^{abcd} \nabla_c \xi_d + 4 \xi_d \nabla_c \text{eof}^{abcd}$ , which we calculate separately and add together below.

```
In[13]:= xi1 = {1, 0, 0, 0, 0};
xiD = lower[%];
dxi = covariant[%];
tr[-2 eof ** dxi, {3, 5}, {4, 6}] // Simplify;
                                         化简

%[[1, 2]] * 2 Pi^2 * r^3;
                                         圆周率

qXiPart1 = % // Simplify;
                                         化简
```

```
In[19]:= lower[eof, {1, 2, 3, 4}];
covariant[%];
contract[%, {1, 5}];
raise[%, {1, 2, 3}];
-4 %.xiD;
%[[1, 2]] * 2 Pi^2 * r^3;
                                         圆周率

qXiPart2 = % // Simplify;
                                         化简
```

```
In[26]:= qXi = qXiPart1 + qXiPart2 // Simplify;
                                         化简

qXi = % /. f -> fff // FullSimplify;
                                         完全简化

dQ = tDelta[qXi] // Simplify;
                                         化简
```

(2) We calculate  $-\int \xi \cdot \Theta$  below: the minus sign has been considered implicitly below. In higher curvature gravity,  $\Theta^a = 2 \text{eof}^{abcd} \nabla_d \delta g_{bc} - 2 \nabla_d \text{eof}^{abcd} \delta g_{cd}$ . We calculate the two parts separately and add them together.

```
In[29]:= dMetric[r_] = {{ad[r], 0, 0, 0, 0}, {0, bd[r], 0, 0, 0},
                        {0, 0, 0, 0, 0}, {0, 0, 0, 0, 0}, {0, 0, 0, 0, 0}};
ddMetric = covariant[dMetric[r]];
adf[r_] = tDelta[-fff[r]];
bdf[r_] = tDelta[1 / fff[r]];
```



```
In[33]:= 2 tr[ef.ddMetric, {2, 4}, {3, 5}] // Simplify;
```

化简

```
xiThetaPart1 = %[[2]];
xiTheta1 = % * 2 Pi^2 r^3;
```

圆周率

```
In[36]:= lower[ef, {1, 2, 3, 4}];
covariant[%];
contract[%, {1, 5}];
-2 * % ** dMetric[r];
contract[%, {2, 4}, {3, 5}];
xiThetaPart2 = %[[2]];
xiTheta2 = % * 2 Pi^2 r^3;
```

圆周率

```
In[43]:= xiTheta = xiTheta1 + xiTheta2 // Simplify;
```

化简

```
xiThetaT = xiTheta /. {f -> fff, ad -> adf, bd -> bdf} // Simplify;
```

化简

(3) Adding the results from (1) and (2) together, one gets  $\int \delta Q - \xi \cdot \Theta$  for the Killing vector  $\xi_t$  in the present case. Then regularize it by subtracting the results for the pure AdS. (The substitution  $\{M \rightarrow 0, dM \rightarrow 0\}$  below gives the pure AdS result directly; alternatively, one can repeat the above calculation again starting from the metric of pure AdS obtained from  $M=0$ .)

```
In[45]:= dQ + xiThetaT // Simplify;
```

化简

```
dqXi = Coefficient[%, dM] dM + Coefficient[%, dl] dl + Coefficient[%, dα] dα
```

系数

系数

系数

Out[46]=

$$dM + \frac{3 dl \pi r^4}{4 l^3} + \frac{1}{32 \alpha^2} d\alpha$$

$$\left( -32 M \alpha + 3 \pi r^4 \left( -5 + \frac{20 \alpha}{l^2} \right) + \frac{15 \pi^{3/2} r^6 (l^2 - 8 \alpha)}{1 \sqrt{-8 \pi r^4 \alpha + l^2 \left( \pi r^4 + \frac{64 M \alpha}{3} \right)}} + \frac{192 l M r^2 \alpha}{\sqrt{-8 r^4 \alpha + l^2 \left( r^4 + \frac{64 M \alpha}{3 \pi} \right)}} \right)$$

In[47]:=

```

dQXi;
% /. {M -> 0, dM -> 0};
Limit[Simplify[% - %], r -> Infinity];
极限 化简 无穷大
dQXiReg = Coefficient[%, dM] dM + Coefficient[%, dl] dl + Coefficient[%, dα] dα
系数 系数 系数

```

Out[50]=

$$dM + \frac{d\alpha M \left( -1 + \frac{1}{\sqrt{1^2 - 8\alpha}} \right)}{\alpha}$$

Thus, we identify  $\Delta V_{GB} = \frac{M}{\alpha} \left( 1 - \frac{1}{\sqrt{1 - \frac{8\alpha}{l^2}}} \right)$  and  $\Delta V = 0$ . And for later usage, we

define

In[51]:=

$$\text{deltaV2} = \frac{M}{\alpha} \left( 1 - \frac{1}{\sqrt{1 - \frac{8\alpha}{l^2}}} \right);$$

(4) **Verification of the extended first law.** Below the expressions of  $M$ ,  $T$ ,  $S$ ,  $V$ ,  $V_\alpha$  are denoted by  $mh$ ,  $tem$ ,  $entr$ ,  $vol0$ ,  $vol2$ . When verifying the extended 1st law, we use the outer horizon radius  $r_h$ , the cosmological constant  $\Lambda$  and the couplings  $\alpha$  as independent variables.

The expressions of the thermodynamic quantities are listed below:

In[52]:=

$$\begin{aligned}
mh &= \frac{3\pi rh^2}{8} + \frac{3\pi rh^4}{8l^2} + \frac{3\pi\alpha}{4}; \\
tem &= \frac{l^2 rh + 2rh^3}{2l^2\pi rh^2 + 8l^2\pi\alpha}; \\
entr &= \frac{\pi^2 rh^3}{2} + 6\pi^2 rh\alpha;
\end{aligned}$$

```
In[55]:= 2 Pi^2 r^3;
          [圆周率]
int[r_] = Integrate[%, r];
          [积分]
- (int[r] - int[rh]) + (int[r] /. M -> 0);
Limit[%, r -> Infinity];
[极限]      [无穷大]
vol0 = %
```

```
Out[59]= 
$$\frac{\pi^2 r h^4}{2}$$

```

```
In[60]:= 1 / (16 Pi) (norm[rie0] - 4 norm[RicciTensor] + (RicciScalar)^2) // Simplify;
          [圆周率]                                     [化简]
% * 2 Pi^2 r^3 /. {f -> fff} // Simplify;
          [圆周率]                                     [化简]
Integrate[%, r];
[积分]
int[r_] = %;
- (int[r] - int[rh]) + (int[r] /. M -> 0);
Limit[%, r -> Infinity];
          [无穷大]
vol2 = %;
```

Verification of the extended first law :

```
In[67]:= va = {rh, 1, α};
For[i = 1, i ≤ 3, i++, Print[Simplify[D[mh, va[[i]]] -
[For循环]      [打印]      [化简]      [偏导]
    tem * D[entr, va[[i]]] - (vol0 /. M -> mh) * D[(-  $\frac{\Lambda}{8 \text{ Pi}}$  /. Λ -> -  $\frac{6}{1^2}$ ), va[[i]]] -
    [偏导]      [偏导]
    ((vol2 + deltaV2) /. M -> mh) D[α, va[[i]]] ] == 0]
    [偏导]
]]
```

True

True

True

Below is another verification by comparing with existing literature. In the first line, we obtain the thermodynamic volume conjugate to  $\alpha$  from eq.(2.23) in arXiv:1406.7015. In the second line, we present our result. One can observe that the outcomes are the same, omitting the unimportant constant factor.

```
In[69]:= const rh^(D1 - 2 k) / (16 Pi) (1 / rh -  $\frac{4 \text{ Pi } k T}{D1 - 2 k}$ ) /. {k → 2, D1 → 5, T → tem} // Simplify
      [圆周率] [化简]

((vol2 + deltaV2) /. M → mh) // Simplify
      [化简]
```

```
Out[69]=
```

$$-\frac{\text{const} (8 \text{ rh}^4 + 1^2 (3 \text{ rh}^2 - 4 \alpha))}{16 1^2 \pi (\text{rh}^2 + 4 \alpha)}$$

```
Out[70]=
```

$$-\frac{3 \pi (8 \text{ rh}^4 + 1^2 (3 \text{ rh}^2 - 4 \alpha))}{4 1^2 (\text{rh}^2 + 4 \alpha)}$$

(5) Verification of the correlation between the additional terms  $\Delta M = M - M_K$  and  $\Delta V_n$ , as suggested in the paper.

The Komar mass  $M_K$  and the term  $\Delta M$  are calculated as

```
In[71]:= (D1 - 2) / (D1 - 3) qXi /. D1 → 5;
% /. M → 0;
%% - % // Simplify;
      [化简]

MK = Limit[%, r → Infinity];
      [极限] [无穷大]

deltaM = M - MK // Simplify
      [化简]
```

```
Out[75]=
```

$$M - \frac{1 M}{\sqrt{1^2 - 8 \alpha}}$$

Then verify the correlation between the additional terms  $\Delta M = M - M_K$  and  $\Delta V_n$  as below.

```
In[76]:= deltaM == deltaV2 * alpha // FullSimplify
      [完全简化]
```

```
Out[76]= True
```

(6) One can use the effective cosmological constant  $\Lambda_e$  (or the effective AdS radius denoted by  $l_e$ ) to rewrite the first law.

In[77]:=

```
fff[r] /. M -> 0;
% == 1 +  $\frac{r^2}{le^2}$ ;
Solve[%, l][[2]] // Simplify
解方程 化简
```

Out[79]=

$$\left\{ l \rightarrow \frac{le^2}{\sqrt{le^2 - 2\alpha}} \right\}$$

Thus we get the relationship between the AdS radius  $l$  (its expression is denoted as  $lf$ ) and the effective AdS radius  $le$  (its expression is denoted as  $lef$ ), as given by

In[80]:=

$$lf = \frac{le^2}{\sqrt{le^2 - 2\alpha}}; \quad lef = \frac{\sqrt{1^2 + \sqrt{1^2 (1^2 - 8\alpha)}}}{\sqrt{2}};$$

If one would like to use  $\Lambda e$  as the variable in the extended first law,  $dl$  can be replaced by terms proportional to  $dle$  and  $d\alpha$  like this:

In[81]:=

```
dlf = D[lf, le] dle + D[lf, α] dα // Expand
偏导 偏导 展开
```

Out[81]=

$$\frac{d\alpha le^2}{(le^2 - 2\alpha)^{3/2}} - \frac{dle le^3}{(le^2 - 2\alpha)^{3/2}} + \frac{2 dle le}{\sqrt{le^2 - 2\alpha}}$$
